# Supplementary material for: Context-based navigation for ground mobile robot in a semi-structured indoor environment
Source: arXiv:2111.12111 source file (2021-11-23)
Supplement: Supplementary file 1 [file AdditionalText.tex]

\subsection{Knowledge}
        The knowledge contains information about the possible configurations of the robot components. It is implemented using OWL, the Web Ontology Language. An advantage of using OWL is that a off the shelf reasoner can be used \cite{Sirin2007Pellet:Reasoner}.
    
    \subsection{Monitor}
        The observers (rosgraph\_monitor) monitor the runtime context and the quality attributes of the current configuration. The observers are used to detect multiple different events: mis-configured parameters, erroneous behavior of components, violation of system requirements, and the level of the quality attributes. The information that is determined by the observers is used to update the knowledge base. This updated information is then used by other components in the framework.

    \subsection{Analyse, Plan}
        The update information is used by the mros\_reasoner to check if the current objectives and the non-functional requirements are met. The mros\_reasoner is an ontological reasoner, and uses SWRL rules to reason using the knowledge base ontology.
        
        If the reasoner finds an objective violation, the plan phase will be triggered. In that case, a search is done for the best alternative configuration that complies with the objectives and the non-functional requirements. This step is executed in the mros\_reasoner as well, using ontology search queries.
    
    \subsection{Execute}
        If a new system configuration is desired and found by the reasoner, the rosgraph\_manipulator is triggered. This node will launch the new configuration. Since ROS1 does not have life cycle management, the old configuration will be killed before the new configuration can be launched. Life cycle management is an huge improvement with ROS2, which makes it easier to switch to other configurations.

% The MROS framework is used as a tool to obtain the self-adaptation capabilities. This framework follows the MAPE-K philosophy. The quality and environment observers and the quality models, which are developed in this research, are implemented in this framework. Final experiments are set-up to test the framework with the quality models. 
 
 For the benchmark, a robot system without metacontroller is used: a fixed configuration.

%\section{MROS implementation}
%The MROS framework is used as a tool to obtain the self-adaptive capabilities. This framework follows the MAPE-K philosophy. The quality and environment metrics and the quality models, which are developed in this research, are implemented in this framework. 

 \section{MROS implementation}

The last research sub-question in answered in this chapter: \textit{How can the predicted quality models be used in a self-adaptive framework, in order to improve the overall navigation quality?} First the general concept of the MROS framework is analysed. Next, the implementation of the new (sub)components is explained, including the interface with the rest of the framework. Different modifications of the MROS framework are developed, to test different ways of how the quality models can be used in this framework.

\section{MROS, default framework}
    \textcite{HernandezCorbato2020MROS:Architectures} state that the most important feature that differentiates MROS with respect to other frameworks is the strict separation of concerns. The model-based meta controller and the application logic are separated. The meta-controller ensures that the available configurations fulfill the objectives that are commanded by the application logic.
    
    "The MROS meta-controller is responsible for the runtime configuration of the managed application, adapting it according to the non-functional requirements defined at design time and to the dynamically changing context at runtime. It is a managing component that ensures that at each instant the most suitable configuration to realize the present task is activated; accounting for contingencies such as component failures or environment perturbations that affect expected quality attributes."
    
    The MROS framework follows the MAPE-K feedback loop concept \cite{Kephart2003TheComputing}. The working principle of the MROS framework is explained following the MAPE-K loop phases (see figure \ref{fig:mros_overview}).

    \begin{figure}[h!]
        \centering
        \includegraphics[width=0.45\linewidth]{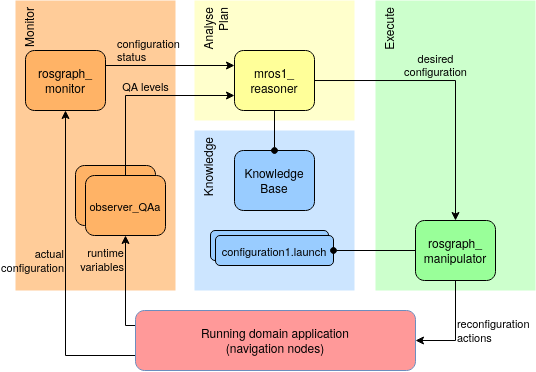}
        \caption{Not up to date! Overview of the MROS framework.}
        \label{fig:mros_overview}
    \end{figure}
    
    \subsection{Knowledge}
        The knowledge base contains the set of possible configurations of the components, and their quality attributes. The knowledge base conforms to the TOMASys ontology, the run-time model which contains the functional information about the managed system, the non-functional requirements, and the objectives. 
        
        The knowledge base is implemented using OWL, the Web Ontology Language. An advantage of using OWL is that a off the shelf reasoner can be used \cite{Sirin2007Pellet:Reasoner}.
    
    \subsection{Monitor}
        The observers (rosgraph\_monitor) monitor the application runtime context and the quality attributes of the current configuration. The observers are used to detect multiple different events: mis-configured parameters, erroneous behavior of components, violation of system requirements, and the level of the quality attributes. The information that is determined by the observers is used to update the knowledge base. This updated information is then used by other components in the framework.

    \subsection{Analyse, Plan}
        The update information is used by the mros\_reasoner to check if the current objectives and the non-functional requirements are met. The mros\_reasoner is an ontological reasoner, and uses SWRL rules to reason using the knowledge base ontology.
        
        If the reasoner finds an objective violation, the plan phase will be triggered. In that case, a search is done for the best alternative configuration that complies with the objectives and the non-functional requirements. This step is executed in the mros\_reasoner as well, using ontology search queries.
    
    \subsection{Execute}
        If a new system configuration is desired and found by the reasoner, the rosgraph\_manipulator is triggered. This node will launch the new configuration. Since ROS1 does not have life cycle management, the old configuration will be killed before the new configuration can be launched. Life cycle management is an huge improvement with ROS2, which makes it easier to switch to other configurations.

\section{MROS, modified framework}
    The implementation of quality models and the other new components are explained in this section. The difference between the new and the default MROS system are analysed per phase in this section, and visualized in figure \ref{fig:systemoverview}.
    
    \begin{figure}[b!]
        \centering
        \includegraphics[width=0.5\linewidth]{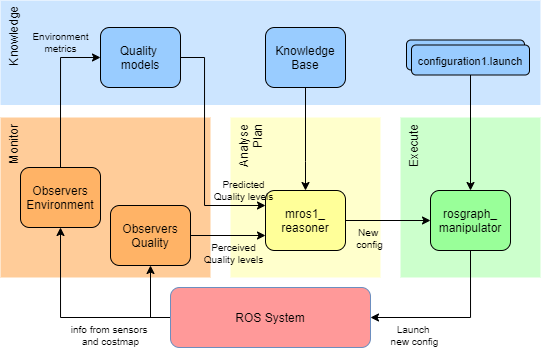}
        \caption{Overview of the implemented self-adaptive system, following the MAPE-K approach}
        \label{fig:systemoverview}
    \end{figure}
    
    \subsection{Knowledge} 
        The knowledge base ontology is equal to the default MROS ontology, build upon the TOMASys ontology. The configuration launch files in the knowledge base are updated with the new configurations. Next to this ontology and the launch files, the quality models are also implemented as knowledge. A separate rosnode is created, where the quality models can be loaded in when the robot in launched. This rosnode will subscribe to the topics where the observers are publishing in, and will predict on request the updated quality levels of the configurations.
    
    \subsection{Monitor} 
        Next to the quality observers that will monitor the current safety and performance levels, environment observers are implemented as well. These environment observers will monitor the environment, using data from the robot's sensors, and determine the Obstacle Density and Narrowness levels.
    
    \subsection{Analyse, Plan} 
        The mros\_reasoner is used again, but some modifications are made. These modification are needed to implemented the quality models, and to research how the quality models can be used. This is in more detail explained in section \ref{mros_mods}.
    
    \subsection{Execute} 
        The rosgraph\_manipulator is not modified. The only difference is that the launch files of new configurations are used.

\section{MAPE-K phase times}
    It can be important to know what the time delays of each step are. The time each phase takes is measured in ROS time and shown in table \ref{tab:mros_times}. ROS time is used since this is considered more relevant than real time, since ROS time is what the robot experiences. The simulation runs on average at 0.8 times real time, so times can easily be converted.
    
    In the analyse phase, the violation of the nfr is checked using the OWL reasoner. This is the second longest phase, with a time of 520ms.
    
    In the plan phase, a new configuration is searched for and this takes only 1ms, and updating the predicted QA levels in the knowledge base using the quality models takes 15ms.
    
    The execution phase is the phase that takes the longest time, and takes 3575ms. In this phase, move\_base of the old configuration is killed, and re-launched with a new configuration. 
    
    \begin{table}[h!]
        \centering
        \caption{The time (ROS time!) each MAPE-K phase takes. (Intel Core i9-9900K @ 4.7 GHz)}
        \label{tab:mros_times}
        \begin{tabular}{l|llll}
                        & Monitor  & Analyse & Plan  & Execute \\ \hline
        Default MROS    & 97        & 520ms   & 1ms   & 3575ms  \\
        Modified MROS   & 97        & 520ms   & 16ms    & 3575ms 
        \end{tabular}
    \end{table}

\section{Reasoner flow modifications} \label{mros_mods}

    \subsection{Mod0: Default MROS system.} 
        This is the default MROS system. The knowledge base is updated with the configurations of this research. The QA values in the knowledge base are initialized with the average values from the experiments, see table \ref{tab:avqa_dwa} and \ref{tab:avqa_teb}. 
        
        The reasoner flow of the default MROS system is displayed in figure \ref{fig:flow_m0}. When a configuration is violating the NFRs, this configuration gets an objective error and cannot be used again. This is because of the functional errors where the framework is designed for. Next the list of function design that are not in error, are used to find the suitable function designs; the configurations that meet the NFRs. When no configurations meet the NFRs, no adaptation takes place. When more than one configurations meet the NFRs, a utility function is used. Right now the utility function only uses the estimated performance levels, the configuration with the highest estimated performance level is selected. This configuration is the new desired configuration.

    \subsection{Mod1: MROS with quality models.}
        This is an updated version of the default MROS reasoner flow, and the quality models are implemented. The reasoner flow is displayed in figure \ref{fig:flow_m1}.
        
        Again, first it is tested if the NFRs are violated. If this is the case, the quality models are used to update the predicted safety values in the knowledge base. The reasoner now has more information than the default MROS system. It is not needed anymore to remove the configurations that once were in violation, since it can be predicted if they will be in error now. 
        
        From the list of configurations that meet the NFRs, the one with the highest performance is selected, equal to the default MROS flow. But when there are no configurations that meet the NFRs, the configuration with the highest safety level is selected. This is done since this will improve the safety level, and therefore the navigation quality. This different than what the default MROS system would do, since the default system would not adapt in this case.
        
    \subsection{Mod2: MROS with quality models, and new adaptation rules}
        The second modification is an update over the first modification, the mod2 reasoner flow is displayed in figure \ref{fig:flow_m2}. 
        
        The only difference with the first modification is that in the case that the NFRs are not in violation, still adaptation can take place. In this case, it is checked if the system can switch back to the initial configuration. Since it is assumed that the system is launched with an initial configuration that is the desired configuration, and therefore this option is investigated. The initial configuration is usually the fastest configuration. If the system is able to switch back to the fast configuration, the average performance level will be improved. The system will always use this fast configuration, except when the safety level is below the requirement.
        
        \begin{figure}[h!]
            \centering
            \includegraphics[height=9cm]{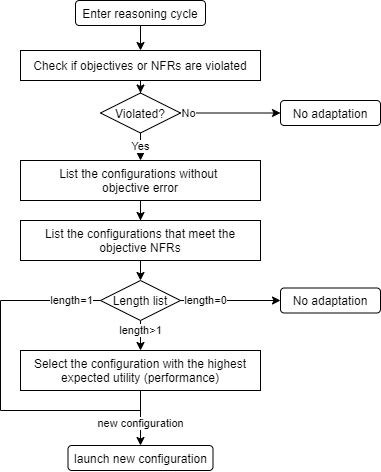}
            \captionof{figure}{Reasoner flow MROS default (m0).}
            \label{fig:flow_m0}
        \end{figure}
        \begin{figure}[h!]
            \centering
            \includegraphics[height=9cm]{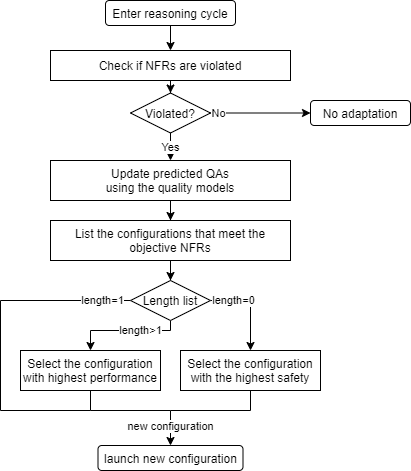}
            \captionof{figure}{Reasoner flow modification 1.}
            \label{fig:flow_m1}
        \end{figure}
        \begin{figure}[h!]
            % \centering
            \includegraphics[height=9cm]{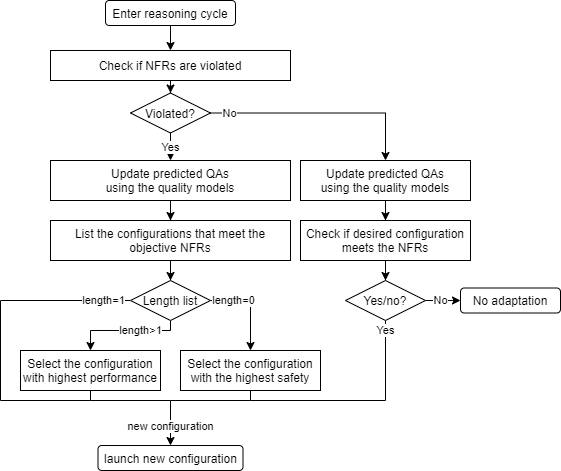}
            \caption{Reasoner flow modification 2.}
            \label{fig:flow_m2}
        \end{figure}

    \newpage
\section{Discussion of results}
    Modification 0 does not use the quality models. This system cannot predict which configuration will be in error. Therefore. the system just chooses the next best configuration, based on the average safety and performance levels from the knowledge base. It can be case, however, that this configuration will also violate the non-functional requirement. This will result in a lower safety level.
    
    Modification 1 does use the quality models. When adaptation is needed, the quality models will update the QA levels in the knowledge base based on the current environment. By doing this, the reasoner knows which configurations will be violating the nfr in the current environment, and can therefore make a better informed choice for adaptation. The result is less violation time and improve average safety. The cost of this is a lower average performance since often a more safe configuration is chosen, which usually has a lower performance.

    Modification 2 is able to switch back to the desired (initial) configuration when there are no NFR violations. The result is a lower average safety compared to mod1, and a higher violation time. This is because, after switching back, in the next unsafe situation that the robot encounters, a less safe configuration is used. But the improvement of this modification is in the performance. Since it is possible to switch back to the faster configuration when the environment allows this, the performance does increase.
    
    To answer the experiment question: it can be concluded that the use of quality models in this self-adaptive framework is indeed useful.
